# Supplementary material for: Optimal Strategies for Matching and Retrieval Problems by Comparing Covariates
Source: arXiv:1807.04834 source file (2018-07-16)
Supplement: Supplementary file 1 [file appendixb.tex]

\section{Appendix: Expected performance based on gender matching} \label{appendixa}
In this appendix we discuss the performance to be expected in the matching and verification tests, when the matching is done based purely on gender. It is to be noted that gender is merely an example here; the analysis can be extended to other covariates.

We assume below that in any distribution of human-subject data, the division of subjects between male and female genders to be half and half. The analysis is, however, easily extended to other proportions.

\subsection{Accuracy of 1:2 matching based on gender}
We show that the equal-error-rate for 1:2 matching can be as high as 25\%, through gender matching alone. 

The problem is as follows:  a probe input (voice or face), and a gallery consisting of two inputs (face or voice), one of which is from the same subject as the probe. We must identify which of the two is the true match.

\subsubsection{Perfect gender identification}
Consider the situation where we are able to identify the gender of the subject of the data (face or voice) perfectly.

There are two possibilities: (a) both probe instances are the same gender, and (b) they are different genders.  Each of the two possibilities occurs with a probability of 0.5

We employ the following simple strategy: If the two gallery instances are different genders, then we select the instance whose gender matches the probe. In this case, clearly, the probability of error is 0.  If the two instances are the same gender, we select one of them randomly with a probability of 0.5.  The probability of error here is 0.5.

Thus, the overall probability of error is 
\[
Prob(error) = 0.5 \times 0 + 0.5 \times 0.5 = 0.25.
\]

\subsubsection{Imperfect gender identification}
Now let us consider the situation where gender identification itself is imperfect, and we have error rates $e_f$ and $e_v$ in identifying the gender of faces and voices, respectively.  Assume the error rates are known.  We will assume below that gallery entries are faces, and probe entries are voices. (The equations are trivially flipped to handle the converse case).

Since we are aware that we sometimes make mistakes in identifying gender, we modify our strategy as follows: when the gallery items are found to have mismatched gender, we select the entry with the same gender as the probe only $P$ of the time (so that if the gender classification was correct, we would have a match error rate of (1-$P$)). When both gallery items are found to be the same gender, we choose randomly.

The actual error can now be computed as follows. The gallery items are both of the same gender in 0.5 of the trials, and of mismatched gender in the remaining 0.5 of the trials.

When both gallery items have the same gender, regardless of the strategy chosen, the probability of error is 0.5 (by symmetry). 

When both gallery items are of mismatched gender, we have 8 combinations of correctness of gender-classification. Table \ref{error_prob} lists all eight, along with the probability of matching error (in the final column). 
\begin{table}[ht]
	\centering
	
	\footnotesize
	\begin{tabular}{c|c|c|c|c}
		\hline
		type & probe & gallery1 & gallery2 & $Prob(error,type)$ \\
		\hline
		1 & \checkmark & \checkmark & \checkmark & $(1-e_v)(1-e_f)^2\cdot(1-P)$ \\
		2 & \checkmark & $\times$ & \checkmark & $(1-e_v)e_f(1-e_f)\cdot 0.5$ \\
		3 & \checkmark & \checkmark & $\times$ & $(1-e_v)(1-e_f)e_f\cdot 0.5$ \\
		4 & \checkmark & $\times$ & $\times$ & $(1-e_v)(e_f)^2\cdot P$ \\
		5 & $\times$ & \checkmark & \checkmark & $e_v(1-e_f)^2\cdot P$ \\
		6 & $\times$ & $\times$ & \checkmark & $e_{v}e_f(1-e_f) \cdot 0.5$ \\
		7 & $\times$ & \checkmark & $\times$ & $e_v(1-e_f)e_f \cdot 0.5$ \\
		8 & $\times$ & $\times$ & $\times$ & $e_v(e_f)^2\cdot (1-P)$ \\
		\hline
	\end{tabular}
	\caption{\footnotesize the possible error types with probabilities.}\label{error_prob}
\end{table}
Taking type 1 as an example, we have probability $(1-e_v)(1-e_f)^2$ that the gender of both probe and galleries are correctly classified. In this case, our strategy gives us an error of $(1-P)$. For type 2, the gender of probe and one of the gallery items is correctly classified, while the other gallery item is misclassified, we have an error of 0.5. If we go through all the cases, the total error $Prob(error)$ can be computed as 
\begin{equation*}
\begin{split}
Prob(error) =  0.25 + 0.5\sum_{type=1}^{8} Prob(error,type) \\
= 0.25+0.5(2e_{f}e_v - e_v - e_f + 1 \\
+ P(2e_f + 2e_v - 4e_{f}e_v - 1))
\end{split}
\end{equation*}

Our objective is to minimize $Prob(error)$, so we must choose $P$ to minimize the above term. I.e. we must solve
\[
\begin{split}
&\arg\min_{P} \ 2e_{f}e_v - e_v - e_f + 1 + P(2e_f + 2e_v - 4e_{f}e_v - 1)\nonumber\\
&{\mathrm s.t.} \ \ 0\leq P\leq 1. \nonumber
\end{split}
\]
Its easy to see that the solution for $P$ is 1.0 if its multplicative factor is negative in the above equation, and 0 otherwise. {\em i.e.}
\begin{equation*}
P = 
 \begin{cases}
      1, & \text{if}\ e_f + e_v < 2e_{f}e_v + 0.5 \\
      0, & \text{else}
    \end{cases}
\end{equation*}
The corresponding match error rates are $Prob(error) = 0.25+0.5(e_f+e_v - 2e_ve_f)$ and $0.75+e_fe_f - 0.5(e_v + e_f)$ respectively.

Although complicated looking, the solution is, in fact, quite intuitive.  When gender classification is either better than random for both modalities ({\em i.e.} $e_f,e_v > 0.5$) or worse than random for both ($e_f, e_v < 0.5$), the best strategy is to select the gallery item that matches the gender of the probe.  If either of these is random ({\em i.e.} either $e_f$ or $e_v$ is 0.5) , the choice of $P$ does not matter, and the error is 0.5. If one of the two is correct more than half the time, and the other is wrong more than half the time ({\em e.g.} $e_f < 0.5,~e_v > 0.5$), the optimal choice is to select the gallery item that is classified as {\em mismatched} in gender with the probe.

\subsection{Accuracy of 1:$N$ matching based on gender}
We now consider the best achievable performance on 1:$N$ matching, when the only information known is the gender of the voices and faces. 
\subsubsection{Perfect gender identification}
Consider the situation where the gender of the faces and voices in each test trial is perfectly known.

We employ the following strategy: we randomly select one of the gallery instances that have the same gender as the probe instance. If there are $K$ {\em imposter} gallery instances of the same gender as the probe instance, the expected {\em accuracy} is $\frac{1}{K+1}$. The probability of randomly having $K$ of $N-1$ imposters of the same gender as the probe is given by 
\[
Prob(K;N-1) = {{N-1}\choose{K}} 0.5^{N-1}
\]
The overall accuracy is given by:
\begin{align*}
Prob(correct) &= \sum_{k=0}^{N-1}\frac{Prob(k;N-1)}{k+1} \\
&= 0.5^{N-1}\sum_{k=0}^{N-1} {{N-1}\choose{K}}\frac{1}{k+1} \\
&=  \frac{0.5^{N-1}}{N} \sum_{k=1}^N {{N}\choose{k}} \\
&= \frac{0.5^{N-1} (2^N - 1)}{N} \\
&= \frac{(2 - 0.5^{N-1})}{N},
\end{align*}
giving us the error
\[
P(error) = 1 - \frac{(2 - 0.5^{N-1})}{N}.
\]

\subsection{EER of verification based on gender}
Here we show that the equal-error-rate for verification (determining if the the subjects in two recordings are the same) can be as high as 33\%, through gender matching alone. 

The problem is as follows:  we are given a pair of inputs, one (features extracted from) a face, and the other a voice.  We must determine whether they are both from the same speaker.

The test set include some number of ``positives'', where both do belong to the same subject, and some ``negatives'', where both do not.  If a positive is falsely detected as a negative, we have an instance of false rejection.  If a negative is wrongly detected as a positive, we have an instance of false acceptance.

Let $F_R$ represent the `false rejection rate'', i.e. the fraction of all positives that are wrongly rejected. Let $F_A$ represent the ``false acceptance rate'', i.e. the fraction of negatives that are wrongly accepted. Any classifier can generally be optimized to trade off $F_R$ against $F_A$. The ``Equal Error Rate'' (EER) is achieved when $F_R = F_A$.

Among the ``positive'' test pairs, both voice and face in each pair have the same gender. We assume the ``negative'' test instances are drawn randomly, {\em i.e.}, 0.5  of all negative pairs have the same gender, while the remaining 0.5 do not.

\subsubsection{Perfect gender identification}
Consider the situation where we know the subject's gender for both the voices and faces (or, alternately, are able to identify the gender from the voice or face perfectly). 

We employ the following strategy:  if the gender of the voice and face are different, we declare it as a negative 100\% of the time.  If the two are from the same gender, we randomly call it a positive $P$ of the time, where $0 \leq P \leq 1.0$.

Using this strategy, the false acceptance rate is:
\begin{equation*}
F_A = 0.5\times 0 + 0.5 \times P = 0.5 P. 
\end{equation*}
Here we're considering that using our strategy we never make a mistake on the 50\% of negative pairs that have mismatched genders,  but are wrong $P$ of the time on the negative pairs with matched genders.

Among the positives, where all pairs are gender matched, our strategy of accepting only a fraction $P$ of them as positives will give us a false rejection rate $F_R = 1-P$.

The equal error rate is achieved when $F_R = F_A$, i.e.
\begin{equation}
0.5P = 1-P, \nonumber
\end{equation}
giving us $P = \frac{2}{3}$, i.e. the best EER is achieved when we accept gender-matched pairs two-thirds of the time.

The EER itself is $0.5P = \frac{1}{3}$.

Thus, merely by being able to identify the gender of the subject accurately, we are able to verification EER of 0.33.

\subsubsection{Imperfect gender identification}
Now let us consider the situation where gender identification itself is imperfect, and we have error rates $e_f$ and $e_v$ in identifying the gender of the face and the voice, respectively. Assume these error rates are known.

To account for this, we modify our strategy:  when we find the genders of the voice and face to match, we accept the pair as positive $P$ of the time,  but when they are {\em mismatched} we still accept them as positive $Q$ of the time.

Let $\alpha$ represent the probability that we will correctly call the polarity of the gender match between the voice and the face. {\em I.e.} $\alpha$ is the probability that if the two have the same gender, we will correctly state that they have the same gender, or if they are of opposite gender, we will correctly state they are of opposite gender.
\[
\alpha = (1 - e_f)(1 - e_v) + e_f e_v. \nonumber
\]
This combines two terms: that we call the genders of both the voice and face correctly, and that we call them both wrongly (which also results in finding the right polarity of the relationship). Its easy to see that $0.5 \leq \alpha \leq 1$, and to verify that when gender identification is perfect, $\alpha = 1.0$.  The probability of calling the polarity of the gender relationship wrongly is $1 - \alpha$.

Among the positive test pairs, all pairs are gender matched. We will correctly call $\alpha$ of these as gender matched. Using our strategy, our error on these instances is $(1-P)$.  We will incorrectly call $1 - \alpha$ of these as gender mismatched, and the error on these instances is $(1 - Q)$.  So the overall false rejection rate is given by
\[
F_R = \alpha(1-P) + (1-\alpha)(1-Q) \nonumber = 1 - \alpha P - (1 - \alpha)Q \nonumber
\]

Among the negative pairs, half are gender matched, and half are gender mismatched. Using the same logic as above, the error on the gender-matched negative pairs is $\alpha P  + (1 - \alpha)Q$. Among the gender mismatched pairs the error is $\alpha Q + (1 - \alpha)P$. The overall false acceptance rate is given by  
\[
F_A = 0.5(\alpha P + (1 - \alpha) Q) + 0.5(\alpha Q + (1 - \alpha)P) = 0.5(P+Q). \nonumber
\]

Equating $F_A$ and $F_R$ as the condition for EER, we obtain
\begin{align*}
&1 - \alpha P - (1 - \alpha)Q = 0.5(P+Q) \\
\Longrightarrow~~~&(3 - 2\alpha)Q + (1 + 2\alpha)P = 2.&\nonumber
\end{align*}

Since at EER,  the EER equals $F_A$, and we would like to minimize it, we obtain the following solution to determine the optimal $P$ and $Q$:
\[
\begin{split}
&\arg\min_{P,Q} P+Q \nonumber\\
&{\mathrm s.t.} 1\geq P,Q\geq 0,~~(3 - 2\alpha)Q + (1 + 2\alpha)P = 2. \nonumber
\end{split}
\]
Its easy to see that the solution to this is obtained at 
\[
\begin{split}
&Q = 0\nonumber\\
&P = \frac{2}{1 + 2\alpha}.\nonumber
\end{split}
\]

That is, the optimal solution is to always reject pairs detected as having mismatched genders, and to accept matched-gender pairs $\frac{2}{1 + 2\alpha}$ of the time. The optimal EER is $\frac{1}{1 + 2\alpha}$.

It is rather straightforward to extend the above analyses to the case when the genders are imbalanced in the test set, and to account for the case where the gender-classification error itself depends on the gender.   We leave this simple, but perhaps tedious extension as an exercise for a later report.
